# Supplementary material for: The Interstate-24 3D Dataset: a new benchmark for 3D multi-camera vehicle tracking
Source: arXiv:2308.14833 source file (2023-08-28)
Supplement: Supplementary file 2 [file oldSupplement.tex]

Appendix I: File Format and Included Files

Appendix II: Links to Videos
All videos are trimmed to include somewhat more frames than the (reported) number of annotated frames for the scene to allow for broader downstream uses.

Appendix III: Scene Homography

Appendix IV: Scene and Timestamp Error and Corrections(Including Description and Examples of Errors)

Appendix V: Vehicle Size Estimation Error Data

Appendix VI: Additional Experimental Settings and Implementation Details

Appendix VII: Full Results

Appendix VIII: Privacy Considerations


\begin{myitem}
        \item \textbf{Roadway curvature} - some camera fields of view contain portions of roadway with slight curvature. In these cases, any planar assumption of x-direction uses a straight axis to explain a curving roadway direction. Small roadway curvature visible over long distances compounds to create large errors in the lateral (y) direction when using a straight-lane assumption for each camera. Notably, a global coordinate system could mitigate this but existing available GPS data is not sufficiently precise, and surveying the roadway was infeasible. We correct for this by fitting a y-offset for each camera field of view as a function of longitudinal (x) position on the roadway.
        \item \textbf{Camera phase} - each camera records frames at the same nominal frequency (30 fps), but out of phase from one another. For any time $t$, the frame from camera $i$ with timestamp closest to $t$ will have timestamp $t+\delta_i$, where $\delta_i$ is distinct for each camera $i$. Thus, annotations in camera $i$'s field of view cannot be directly compared to annotations in camera $j$'s field of view because the annotations record a vehicle's position at different discrete times. To enable direct comparison, we fit 3rd order polynomial splines to each vehicle, which we use to interpolate vehicle positions at arbitrary times.
        \item \textbf{Camera clock time offsets} - due to network time server limitations for clock synchronization of IP cameras on a spatially large network, camera clocks may be out of sync by several tenths of a second relative to a single global clock. That is, two cameras record a discrete event (e.g. vehicles in a specific position) as occurring at two different times. This issue is especially noticeable given the high speed of objects in our dataset (e.g. at 100 ft/s, a .1 second clock offset yields a 10 foot difference in vehicle position). We correct for this by finding the best camera clock offset for each camera, once per scene.
        \item \textbf{Other frame timing issues} - many IP cameras round or truncate reported timestamps to 0.01s precision. Cameras occasionally send the same frame twice (with the same timestamp), and at other times send a frame  taken $2\delta$ from the previous frame but with a timestamp only $\delta$ different from the last. Such issues may be camera firmware-specific, but dropped frames are a common occurrence in field deployments of IP cameras. Most IP cameras operate with a rolling shutter, meaning that the top and bottom halves of an image are captured at different  (on the order of a few milliseconds) times. We correct for these remaining camera timing errors by identifying the best-fit timestamp for each frame within that minimizes the cross-camera vehicle annotation misalignment between overlapping camera fields of view. See Appendix IV.
\end{myitem}

\subsection{Sources of Cross-Camera Error}
\label{sec:errors}

In this section, we identify  sources of error multi-camera annotation error which are partially responsible for the initial metric results listed in Section \ref{sec:analysis}. These sources of error have been of limited consequence to previous multi-camera datasets with a shared tracking space due to their small spatial scale, synchronized sensors and low object speeds \cite{chavdarova2018wildtrack,chavdarova2017deep,liu2017multi,ferryman2009pets2009}. Then, we propose initial solutions for each to enhance the data in terms of each multi-camera metric.

\subsubsection{Roadway curvature}
We note that some scenes contain portions of roadway with slight curvature. In these cases, any planar assumption of x-direction uses a straight axis to explain a curving roadway direction. Small roadway curvature visible over long distances compounds to create large errors in the lateral (y) direction when using a straight-lane assumption for each camera. Notably, a global coordinate system could mitigate this but existing available GPS data is not sufficiently precise, and surveying the roadway was infeasible. 

\subsubsection{Camera time issues}
Four distinct phenomena in our data make determining the time at which a camera frame was captured difficult, despite each camera recording a \textit{timestamp} for each frame. Each must likely be overcome for any dataset relying on tightly space and time-synchronized video from IP camera networks for tracking fast-moving objects. Appendix IV shows examples of each.
\begin{enumerate}
        \item \textbf{Camera phase} - each camera records frames at the same nominal frequency (30 fps), but out of phase from one another. For any time $t$, the frame from camera $i$ with timestamp closest to $t$ will have timestamp $t+\delta_i$, where $\delta_i$ is distinct for each camera $i$. Thus, annotations in camera $i$'s field of view cannot be directly compared to annotations in camera $j$'s field of view because the annotations record a vehicle's position at different discrete times.
        \item \textbf{Camera clock time offsets} - due to network time server limitations for clock synchronization of IP cameras on a spatially large network, camera clocks may be out of sync by several tenths of a second relative to a single global clock. That is, two cameras record a discrete event (e.g. vehicles in a specific position) as occurring at two different times. This issue is especially noticeable given the high speed of objects in our dataset (e.g. at 100 ft/s, a .1 second clock offset yields a 10 foot difference in vehicle position).
        \item \textbf{Camera timestamp quantization} - many IP cameras round or truncate reported timestamps to 0.01s precision. 
        \item \textbf{Skipped and doubled frames} - cameras occasionally send the same frame twice (with the same timestamp), and at other times send a frame  taken $2\delta$ from the previous frame but with a timestamp only $\delta$ different from the last. Such issues may be camera firmware-specific, but dropped frames are a common occurrence in field deployments of IP cameras.
\end{enumerate}

\subsection{Error Correction Methods}
\subsubsection{Roadway curvature lateral correction}
\label{sec:curve-correction}
We attempt to correct for lateral error by fitting a 2nd-order polynomial curve to a solid lane line for each direction of travel in each camera view.  In the uncorrected, straight-line coordinate system, the y-coordinates of the points along this curve will vary for different values of x. We constrain the y-coordinate to be equal along this curve by shifting all points according to the computed curve. Figure \ref{fig:curve} shows the result for a single camera.

\begin{figure}
    \centering
    \includegraphics[width = \columnwidth]{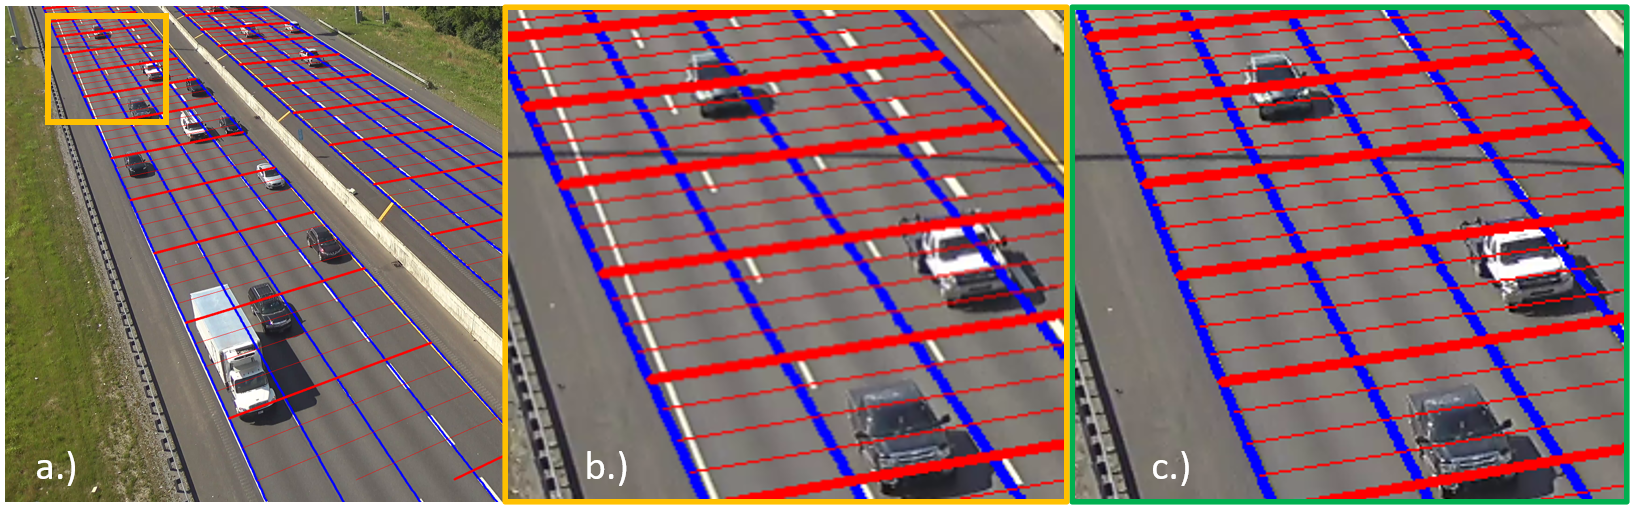}
    \caption{(Left) Before curvature correction, lines in the x-direction (blue) with equal y deviate significantly from roadway direction (white and yellow painted lines on roadway) at distances far from points used to fit local camera homography. (Right) After curvature correction, roadway lines in image have equal y-coordinate. \Derek{Replace with 3 (one original image and 2 bigger subfigures}}
    \label{fig:curve}
\end{figure}

\subsubsection{Camera clock offset correction}
Next, we attempt to correct the camera clock offset. Let the estimate of the true time of frame $j$ for camera $k$ be denoted as $t_{j,k}'$, the reported camera timestamp be $t_{j,k}$the clock offset for camera $k$ be denoted as $o_k$, and the \textit{residual error} due to quantization and skipped/doubled frames for camera $k$ and frame $j$ denoted as $\epsilon_{jk}$. We estimate the true time as:
\begin{equation}
    t_{j,k}' = t_{j,k} + o_k + \epsilon_{j,k}
\end{equation}

Inspired by work on camera synchronization in sports \cite{kumar20113d}, we use vehicles viewed simultaneously by two cameras with overlapping fields of view to estimate the relative clock offset between the two ($o_k$ - $o_k-1$). Let $i$ index the set of $m$ objects  visible in a portion of the roadway coordinate system $[x_{i,min},x_{i,max]}$ in both cameras $k$ and $k-1$. We sample $s$ x-coordinates (indexed by $r$) uniformly spaced across the range $[x_{i,min},x_{i,max]}$. For each point in this range $x_r$, we linearly interpolate between the two closest annotations for camera $k$ to estimate the time at which camera $k$ would have reported object $i$ in position $x_r$. Let $\tau_{r,k}$ denote this time. We set $o_k - o_{k-1}$ to be the mean difference between estimated times of sample x-points from the two cameras.
\begin{equation}
    o_k  - o_{k-1} = \frac{\sum_i \sum_r (\tau_{r,k} - \tau_{r,k-1})}{m*s}
\end{equation}

and set $o_0$ = 0, allowing us to sequentially solve for the rest of camera clock errors. We ignore the effect of quantization for purposes of estimating the camera clock offsets. We assume that the per-camera clock offset does not drift over the relatively short duration of a single scene.

\subsubsection{Quantization and skip frame time correction}
\label{sec:splines}
To reason about the continuous location of an object viewed only through discrete frames at different camera phases, we fit a continuous function to the annotated object locations. Inspired by approaches to trajectory-fitting in \cite{ren2018learning} and \cite{coifman2017critical}, we fit a cubic spline to the x and y positions of vehicle annotations as a function of reported timestamp. Spline-fitting details are given in Appendix V.

We then use the best-fit spline $f_i^{(x)}(t)$ for x-position for each object $i$ visible within frame $j$ of camera $k$ to estimate the residual error for each camera frame $\epsilon_{j,k}$ according to Equation \ref{eq:quant}:

\begin{equation}
    \label{eq:quant}
    \min_{\epsilon_{j,k}} \sum_{i} (w_{i,j,k}(f_{i}^{(x)}(t_{j,k}) - x_{i,j,k}))^2
\end{equation}

where $w_{i,j,k}$ is the change (in pixels) resulting from a 1-foot change in x-position for object $i$ in frame $j$ of camera $k$. We constrain $\epsilon_{j,k}$ to be at most the change associated with a skipped frame ($1/30$s) plus quantization error (0.01s). 

\subsubsection{Annotation shifting}
Thus far, adjustments have only altered timestamps and homography. Further enhancements to vehicle trajectory feasibility can be made by slightly altering the raw annotations at the expense of annotation accuracy within a frame. However, noting that the RMSE for human annotations is 3.12 pixels, we consider small adjustments to raw annotations within this range. We test allowable shifts of 1,2,3, and 5 pixels in the x and y direction separately such that each annotation is moved slightly towards the best-fit spline position at the corresponding time. For each allowable maximum shift, the average shift performed is much smaller (0.25px, 0.36px, 0.42px and 0.47px, respectively).


\section{Enhanced Data Results}
\label{sec:enhanced}

\subsection{Enhanced Multi-Camera Metrics}
Table \ref{tab:metric summary} summarizes all mean metric results for all corrections made. (Error distribution histograms are included in Appendix VII). Corrections are applied sequentially (to data already modified by previous corrections). 

Each correction strictly decrease average errors and increase trajectory feasibility. Curve-correction improves lateral direction cross-camera distance error by 36\% (0.69ft to 0.44ft) and cross-camera pixel error by 16\% (17.6px to 14.8px). Camera clock offset correction decreases average cross-camera distance error in the x-direction by 28\% (2.19ft to 1.58ft) and cross-camera pixel error by an additional 25\%. Offset correction also significantly reduces total variation (1.37 to 1.15) and improves trajectory feasibility by 7.4\%. Residual time error correction further reduces cross-camera distance x-error by an additional 34\% (1.58ft to 1.05ft) relative to the time offset-corrected data. Both timing error corrections almost exclusively effect cross-camera x-error as y varies relatively little with time. We list \textit{Homography} as a baseline and give the CCDE and CCPE for the points used to define the homography themselves; it is unlikely that any correction could reduce error below that threshold without adjusting raw annotations since this error is added to the annotations during homography transformation. 

Subsequent annotation shifting at varying thresholds significantly decreases cross-camera error. A 2-pixel allowable shift (with a corresponding 0.36-pixel average shift across the dataset) improves $CCDE_x$ by 46\% and $CCDE_y$ by 68\%, and also increases trajectory feasibility considerably. This is because annotations are moved towards positions corresponding to a spline fit to data with mostly feasible dynamic assumptions.  Similarly, a 5 pixel maximum allowable shift in each direction reduces $CCDE_x$ by 76\% (1.05 to 0.25 ft) and $CCDE_y$ by 89\% (0.44 to 0.05ft) despite that the average annotation shift is only 0.47 pixels. 


\begin{table}
%\label{tab:metric summary}
\centering
\begin{tabular}{@{}l@{\hskip0.01in}c@{\hskip 0.1in}c@{\hskip 0.1in}c@{\hskip 0.1in}c@{\hskip 0.1in}c@{}}
\toprule
Correction & $CCDE_x$ $\downarrow$ & $CCDE_y$ $\downarrow$ & CCPE $\downarrow$ & $\mathcal{V}_{total}$ $\downarrow$ \\ \midrule
\textit{Homography} & 0.54 ft & 0.18 ft & 3.9 px & -   \\ \midrule
None                & 1.52 ft & 0.69 ft & 17.6 px & 1.37\\
Curve               & 1.52 ft & 0.44 ft & 14.8 px & 1.37\\
Offset              & 1.39 ft & 0.44 ft & 11.1 px & 1.15\\
Residual            & 1.24 ft & 0.44 ft & 7.8 px & 1.11\\ \midrule
1 px shift          & 1.08 ft & 0.26 ft & 5.9 px & 1.08\\
2 px shift          & 0.98 ft & 0.14 ft & 4.6 px & 1.06\\
3 px shift          & 0.91 ft & 0.08 ft & 3.5 px & 1.04\\ 
Spline              & 0.21 ft & 0.04 ft & 1.48 px & 1.03 \\ \bottomrule
\end{tabular}
\caption{All measured metrics for raw annotations and each sequential correction. \Derek{Update text, numbers are good.}}
\end{table}

 Dataset Error Characterization

In this section we analyze the I-24 MC3D dataset single-camera annotation quality, propose metrics to assess the quality of annotations across multiple camera views, and list the initial results for raw data on these metrics which will guide enhancements proposed in Section \ref{sec:errors}.


\subsection{Single-Camera Annotation Quality}
We quantitatively assess annotations  within a single camera field of view in terms of vehicle size accuracy, and variance in human-estimated position.

\subsubsection{Vehicle size accuracy}
We evaluate the accuracy of estimated vehicle sizes based on known vehicle sizes. A subset (10\%) of labeled vehicles within the dataset are selected with discernible make and model. The annotated dimensions for each are compared to the actual size of that vehicle type when available, and otherwise to average vehicle size metrics for that class (semis and trucks). 

Over all sampled vehicles, a mean dimension error of -0.5ft, -0.1ft, and -0.2ft in length, width and height, respectively, was obtained (meaning annotations were too small on average). The standard deviation for each error was 1.1ft, 0.3ft, and 0.6ft respectively. Mean errors for each dimension indicate only slight annotator bias towards undersized annotations, likely due to the difficult of exactly sizing curved 3D vehicles from an oblique angle (notably, vehicles with hard corners such as semis and trucks were not under-estimated). The dimension with the largest distribution of error was length (1.1ft standard deviation).  Full size comparison data is included in Appendix III. 

\subsubsection{Human annotator variance }
We roughly estimate the variance in human-drawn annotations by labeling the same object multiple times for a selection of vehicles. The root mean-squared error (RMSE) is computed for all single-vehicle annotations, and this metric is averaged  across all sampled vehicles to estimate annotator root mean-squared error $RMSE_{ann}$ = 3.12 pixels. This quantity is reported in pixels because the distance-based precision of human annotators varies significantly at different roadway positions.

\subsection{Multi-camera metrics}
\label{sec:raw_metrics}
Relative to I24-MC3D, previous datasets for tracking objects across a shared space \cite{chavdarova2018wildtrack,chavdarova2017deep,liu2017multi} were of relatively small spatial scale, collected with tightly synchronized hardware, and contained slow-moving objects. To address the relative difficulty of multi-camera synchronization in this context, we propose four new metrics that weigh the impact of these challenges in multi-camera tracking data for accurate cross-camera trajectory generation. We define each here and list the computed value for the raw I24-MC3D data:
\begin{enumerate}
    \item \textbf{\textit{Cross-Camera Distance Error}} (CCPE) - the distance (in feet) between two annotations from two different cameras at the same (interpolated) time, when each is projected into roadway coordinate space. This metric indicates the extent to which the annotations can be described by a time-continuous trajectory. Averaged over raw annotations, $CCDE_x$ = 2.19ft and $CCDE_y$ = 0.69ft. By comparison, the $CCDE_x$ = 0.54ft and $CCDE_y$ = 0.18ft for the homography matching points alone, indicating homography is not alone responsible for this error.
    \item \textbf{\textit{Cross-Camera Pixel Error}} (CCPE) - the distance (in pixels) between two annotations from two different cameras at the same (interpolated) time, when one is projected into roadway coordinate space and then into the other image. This metric indicates how useful vehicle annotations from one camera will be when viewed in another camera. Averaged over raw annotations, $CCPE$ = 17.6 pixels, whereas $CCPE$ for homography points is only 3.9px.
    \item \textbf{\textit{Total Variation}} ($\mathcal{V}_{total}$) - the sum of the absolute value of all changes in annotation x-position for a vehicle across increasing annotation time. This metric indicates the smoothness of the trajectory created by assembling all annotations, highly dependent on accurate timestamps for each frame. We compare the ratio of this quantity to the known distance traveled by each vehicle (difference between maximum and minimum x-position) and report this ratio (a ratio of 1 is desired). For raw annotations $\mathcal{V}_{total}$ = 1.37. 
\end{enumerate}

\subsection{Error Correction}

A number of known sources of error are present in the dataset associated, primarily associated with IP camera timing limitations. For instance, IP cameras do not record frames in phase with one another, do not have precisely synchronized local clocks (even with conventional network time servers drift on the order of 0.1s are common for some camera firmwares, often truncate reported times to 0.01s, and occasionally skip or duplicate frames. Appendix IV details the approaches used in this work to correct these errors, and Table \ref{tab:corrections} shows the resulting reductions in error achieved after error correction. Correction yields a 20\% and 44\% reduction in x and y cross-camera misalignment error, and a 31\% reduction in cross-camera pixel misalignment. Note that it is unlikely that any correction strategy could reduce misalignment below the error of the homography. Remaining error is explainable by i.) homography error, ii.) human annotator variance, and iii.) imperfections in timestamp-correction methods.
\begin{table}[h]
    \centering
    \begin{tabular}{lccc}
         \toprule
                 & $CCDE_x$ (ft) & $CCDE_y$ (ft) & CCPE (pixels) \\ \midrule
         Before & 1.52          & 0.64          & 13.28  \\
         \textbf{After}   & \textbf{1.24 }         & \textbf{0.36 }         &\textbf{ 9.26}   \\ \midrule
                  Homography  & 0.54          & 0.18          & 3.91   \\ \bottomrule     
    \end{tabular}
    \caption{Cross-camera annotation misalignment before and after correction. Misalignment from homography alone is the ``best possible" misalignment for annotations labeled with this homography.}
    %\label{tab:corrections}
\end{table}



\section{Results}
\label{sec:results}
\begin{figure}
    \centering
    \includegraphics[width=0.7\textwidth]{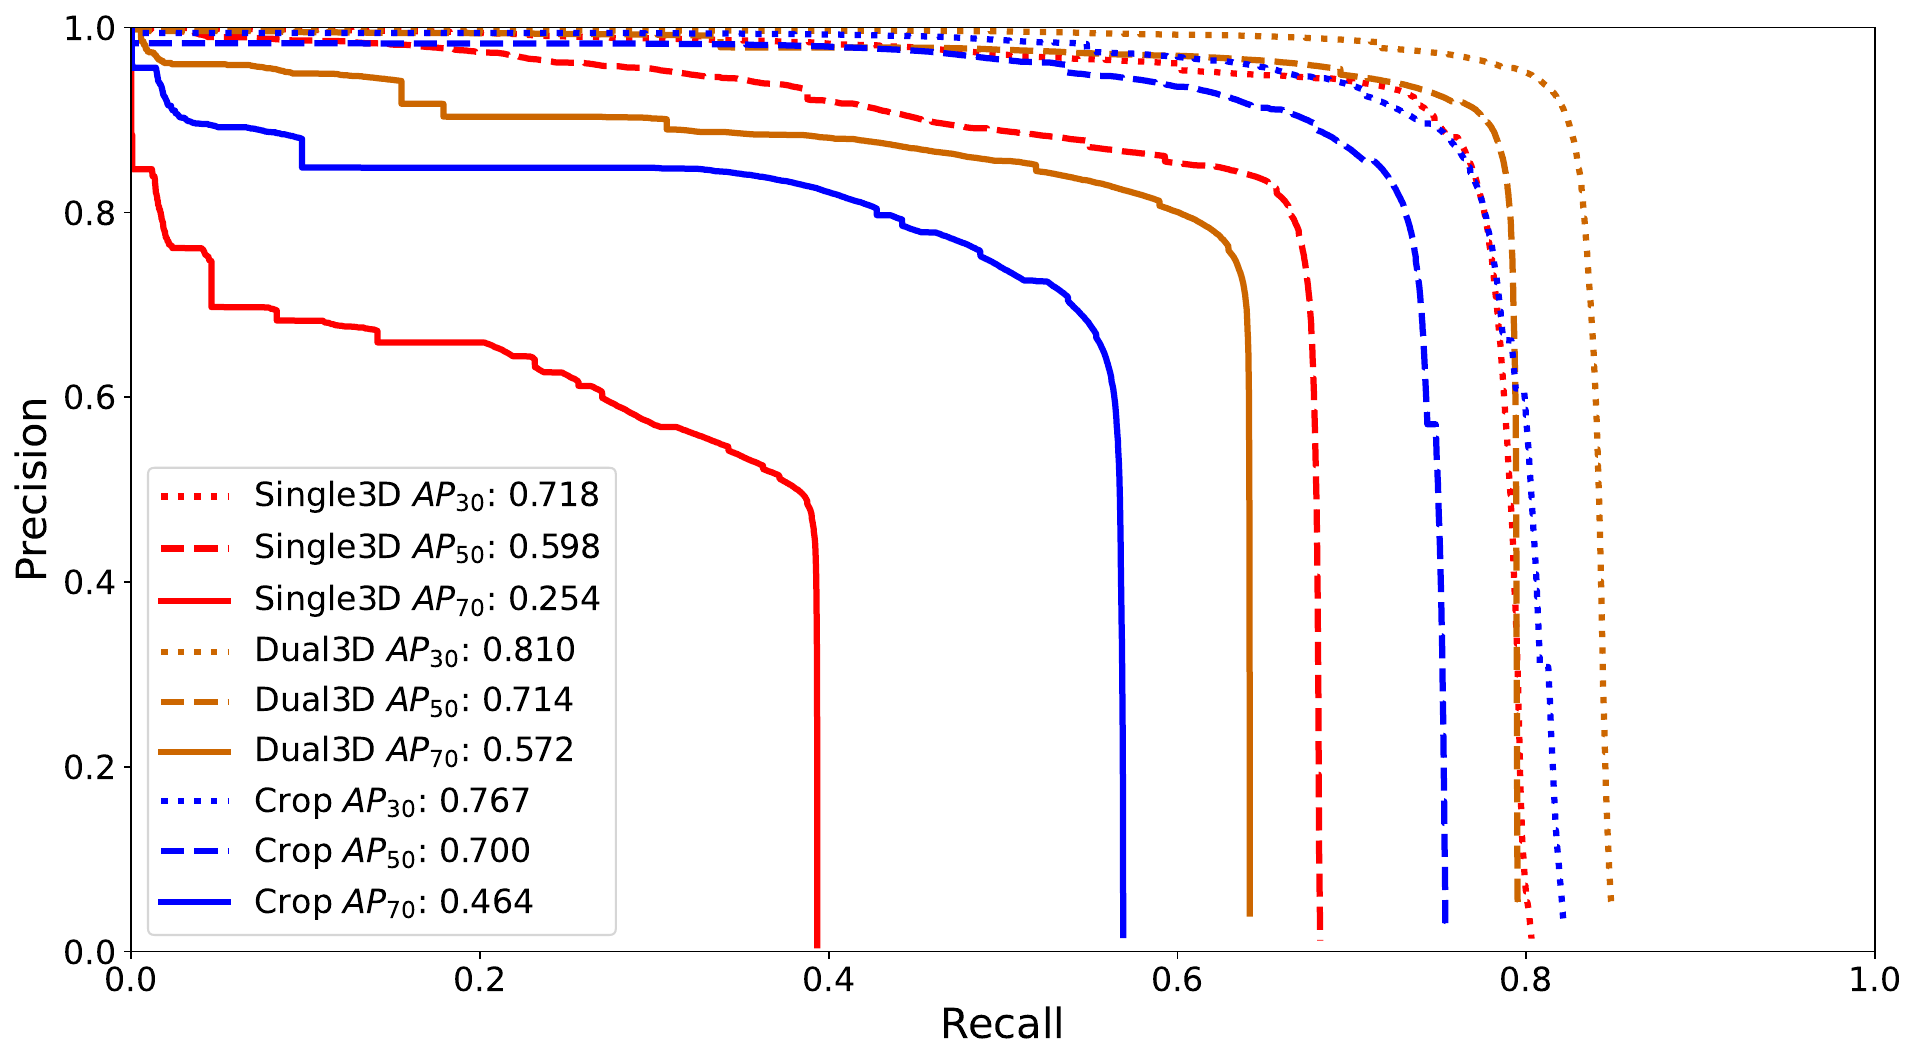}
    \caption{Caption}
    \label{fig:my_label}
\end{figure}



\begin{table}[ht]
\setlength{\tabcolsep}{3pt} % Default value: 6pt
\centering
\begin{tabular}{@{}lcc|ccccccccc@{}} \toprule
 \textbf{Tracker} & \textbf{DF} & \textbf{TF} & \textbf{HOTA} & \textbf{MOTA} & \textbf{Rec} & \textbf{Prec} & \textbf{GT\%} & \textbf{Pred\%} & \textbf{MT} & \textbf{ML} & \textbf{Sw/GT} \\ \toprule
Byte & \checkmark & \checkmark & 51.6 & 85.3 & 87.1 & \textbf{98.0} & 91.7 & \textbf{99.9} & \textbf{72.2} & 3.3 & 0.6 \\
KIOU & \checkmark & \checkmark & 37.4 & 42.6 & 66.3 & 74.7 & 75.3 & 84.1 & 46.2 & 26.8 & \textbf{0.3} \\
Byte &  & \checkmark & \textbf{59.6} & \textbf{86.0} & \textbf{88.9} & 96.8 & \textbf{92.0} & 98.6 & 73.5 & \textbf{2.9} & 0.6 \\
KIOU &  & \checkmark & 44.1 & 45.2 & 68.5 & 75.3 & 78.4 & 84.3 & 49.9 & 21.2 & 0.6 \\ \midrule
Byte & \checkmark &  & 51.4 & 83.6 & 84.0 & 99.8 & 91.9 & 100.0 & 65.5 & 3.3 & 1.3 \\
KIOU & \checkmark &  & 51.1 & 83.6 & 83.9 & 99.8 & 91.9 & 100.0 & 64.4 & 3.8 & 1.3 \\ \midrule
Byte &  &  & 25.6 & 70.0 & 84.7 & 86.3 & 92.0 & 91.4 & 66.6 & \textbf{2.9} & 6.9 \\
KIOU &  &  & 25.6 & 70.0 & 84.7 & 86.3 & 92.0 & 91.4 & 66.6 & \textbf{2.9} & 6.9 \\ \midrule \midrule
\textit{Tracklets} &  & \checkmark & \textbf{61.7} & \textbf{80.8} & 93.6 & \textbf{88.7} & 99.8 & \textbf{96.6} & 91.6 & 1.5 & \textbf{0.5 }\\
\textit{Tracklets} &  &  & 26.0 & 30.1 & \textbf{94.2} & 59.9 & \textbf{100.0} & 81.1 & \textbf{93.7} & \textbf{0.1} & 6.5 \\ \bottomrule
\end{tabular}
\caption{Tracking results for each multi-camera tracking pipeline utilizing ground truth annotations. (Top) GT detections are used within the tracking framework. (Bottom) GT tracklets for each camera field of view are used. Best result for each metric shown in bold.}
\end{table}






 Since ground truth objects are labeled in cameras with varying start times and tracked objects are produced with synchronized timestamps, we compute and compare only the temporally-overlapping sections of each ground truth trajectory dataset with the predictions.
